# Supplementary material for: A Deep Dive into the Distribution Function: Understanding Phase Space Dynamics with Continuum Vlasov-Maxwell Simulations
Source: arXiv:2005.13539 source file (2020-05-27)
Supplement: Supplementary file 1 [file AppendixA.tex]

%Appendix --
\appendix

\chapter{The Dominance of Small Angle Collisions}\label{app:smallAngleCollisions}
