# Supplementary material for: A Deep Dive into the Distribution Function: Understanding Phase Space Dynamics with Continuum Vlasov-Maxwell Simulations
Source: arXiv:2005.13539 source file (2020-05-27)
Supplement: Supplementary file 2 [file AppendixB.tex]

%Appendix
\appendix

\chapter{Multi-Species Model Fokker--Planck Operator}\label{app:multSpeciesModelFP}
