# Supplementary material for: A Deep Dive into the Distribution Function: Understanding Phase Space Dynamics with Continuum Vlasov-Maxwell Simulations
Source: arXiv:2005.13539 source file (2020-05-27)
Supplement: Supplementary file 3 [file AppendixD.tex]

%Appendix
\appendix

\chapter{Counting Noise in Particle-Based Methods}\label{app:noiseParticleMethods}
